# Supplementary material for: On-line Recognition of Handwritten Mathematical Symbols
Source: arXiv:1511.09030 source file (2015-11-29)
Supplement: Supplementary file 1 [file mlp-training.tex]

%!TEX root = "../thesis.tex"

In order to calculate the training rule, we have to take a closer look at the
error function:

\begin{align}
    E_{\Set{x}}(W) &= \frac{1}{2} \sum_{p=1}^{n_\layernumber} {\left ( t_x^{(p)} -o^{(p)}(x) \right )}^2\\
    &= \frac{1}{2} \sum_{p=1}^{n_\layernumber} {\left ( t_x^{(p)} - {(\varphi(\net(x)))}^{(p)} \right )}^2
\end{align}

As only the expression $\net_j$ depends on the weights $w_{j,i}$, one can
simplify the expression by applying the chain rule:

\begin{align}
    \frac{\partial E_{\Set{x}}}{\partial w_{j,i}} &= \frac{\partial E_{\Set{x}}}{\partial \net_j} \frac{\partial \net_j}{\partial w_{j,i}}\\
    &= \frac{\partial E_{\Set{x}}}{\partial \net_j} \frac{\partial \sum_{k \in \text{input neurons}} w_{j,k} x_{j,k}}{\partial w_{j,i}}\\
    &= \frac{\partial E_{\Set{x}}}{\partial \net_j} x_{j,i}
\end{align}

Now we have to calculate $\frac{\partial E_{\Set{x}}}{\partial \net_j}$. At this point, it
is convenient to distinguish two cases. The first one is that $j$ is an output
neuron, the second one is that $j$ is a hidden neuron.

If $j$ is an output neuron, we can use the chain rule again to simplify

\begin{align}
    \frac{\partial E_{\Set{x}}}{\partial \net_j} &=
        \left (\frac{\partial E_{\Set{x}}}{\partial o^{(j)}} \right )
        \left ( \frac{\partial o^{(j)}}{\partial \net_j} \right )\\
    &=  \left ( \frac{\partial}{\partial o^{(j)}} \frac{1}{2} \sum_{p \in outputs} {(t^{(p)} - o^{(p)})}^2  \right )
        \left ( \frac{\partial \varphi(\net_j)}{\partial \net_j} \right )\\
    &=  \left ( \frac{\partial}{\partial o^{(j)}} \frac{1}{2} {(t^{(j)} - o^{(j)})}^2  \right )
        \left ( \frac{\partial \varphi(\net_j)}{\partial \net_j} \right )\\
    &=  -(t^{(j)} - o^{(j)})
        \left ( \frac{\partial \varphi(\net_j)}{\partial \net_j} \right )
\end{align}

Now we have to derive the activation function. If it is the sigmoid function,
we can use \cref{eq:sigmoid-derivate} to continue:

\begin{align}
    \frac{\partial E_{\Set{x}}}{\partial \net_j}
    &=  -(t^{(j)} - o^{(j)}) (o^{(j)} (1 - o^{(j)}))
\end{align}

which leads to

\begin{align}
    \Delta w_{j,i} &= - \eta (-(t^{(j)} - o^{(j)}) (o^{(j)} (1 - o^{(j)})))\\
    &= \eta (t^{(j)} - o^{(j)}) o^{(j)} (1 - o^{(j)})
\end{align}

In the case of weights to hidden layer neurons one can also use chain rule
multiple times:

\begin{align}
    \frac{\partial E_{\Set{x}}}{\partial \net_j}
    &= \sum_{k \in D(j)} \frac{\partial E_{\Set{x}}}{\partial \net_k}
       \frac{\partial \net_k}{\partial \net_j}\label{eq:hidden-layer-update}
\end{align}

Now we define

\[\delta_k := - \frac{\partial E_{\Set{x}}}{\partial \net_k}\]

Note that we already know

\[\delta_k = o^{(k)} (1 - o^{(j)}) (t^{(k)} - o^{(k)}) \;\;\text{ if } k \in outputs\]

So we can continue with \cref{eq:hidden-layer-update}:

\begin{align}
    \frac{\partial E_{\Set{x}}}{\partial \net_j}
    &= \sum_{k \in D(j)} - \delta_k
       \frac{\partial \net_k}{\partial \net_j}\\
    &= \sum_{k \in D(j)} - \delta_k
       \frac{\partial \net_k}{\partial o^{(j)}}
       \frac{\partial o^{(j)}}{\partial \net_j}\\
    &= \sum_{k \in D(j)} - \delta_k
       w_{k,j}
       \frac{\partial o^{(j)}}{\partial \net_j}\\
    &= \sum_{k \in D(j)} - \delta_k
       w_{k,j}
       o^{(j)} (1-o^{(j)})\\
\Leftrightarrow \delta_j &= o^{(j)} (1-o^{(j)}) \sum_{k \in D(j)} \delta_k w_{k,j}
\end{align}
