# Supplementary material for: On-line Recognition of Handwritten Mathematical Symbols
Source: arXiv:1511.09030 source file (2015-11-29)
Supplement: Supplementary file 2 [file perceptron-training.tex]

%!TEX root = "../thesis.tex"

The partial derivative of the \gls{MSE} error function $E$ is calculated like
this:

\begin{align}
    \frac{\partial E}{\partial w^{(j)}} &= \frac{\partial}{\partial w^{(j)}} \frac{1}{2}\sum_{i=1}^m {\left (p_{w, \varphi}(x_i) - y_i \right )}^2\\
    &= \frac{1}{2}\sum_{i=1}^m \frac{\partial}{\partial w^{(j)}} {\left (p_{w, \varphi}(x_i) - y_i \right )}^2\\
    &= \frac{1}{2}\sum_{i=1}^m 2 \cdot (p_{w, \varphi}(x_i) - y_i) \cdot \frac{\partial}{\partial w^{(j)}} \left (p_{w, \varphi}(x_i) - y_i \right )\\
    &= \sum_{i=1}^m (p_{w, \varphi}(x_i) - y_i) \cdot \left ( \frac{\partial}{\partial w^{(j)}} p_{w, \varphi}(x_i) - y_i \right )\\
    &= \sum_{i=1}^m (p_{w, \varphi}(x_i) - y_i) \cdot \left (
            \frac{\partial}{\partial w^{(j)}} \varphi(w^T \cdot x_i) - y_i
        \right )\label{eq:gradient-before-activation-function}
\end{align}

The derivative of the sigmoid function is
\begin{align}
    \frac{\mathrm{d } \sigmoid(x)}{\mathrm{d} x} &= \frac{(1+e^{-x}) \cdot 0 - 1 \cdot \frac{\mathrm{d}}{\mathrm{d}x}(1+e^{-x})}{{(1+e^{-x})}^2}\\
    &= \frac{e^{-x}}{{(1+e^{-x})}^2}\\
    &= \frac{1}{1+e^{-x}} - \frac{1}{{(1+e^{-x})}^2}\\
    &= \sigmoid(x)-{\sigmoid(x)}^2\\
    &= \sigmoid(x) \cdot (1-\sigmoid(x)) \label{eq:sigmoid-derivate}
\end{align}

\paragraph{Now the chain rule is applied  to \cref{eq:gradient-before-activation-function}:}
\begin{align*}
    \frac{\partial E}{\partial w^{(j)}} &= \sum_{i=1}^m (p_{w, \sigmoid}(x_i) - y_i) \cdot \left (
      \sigmoid(w^T \cdot x_i) \cdot (1-\sigmoid(w^T \cdot x_i)) \cdot \frac{\partial}{\partial w^{(j)}} (w^T \cdot x_i)
    \right )\\
    &= \sum_{i=1}^m (p_{w, \sigmoid}(x_i) - y_i) \cdot \left (
      p_{w, \sigmoid}(x_i) \cdot (1-p_{w, \sigmoid}(x_i)) \cdot x_i^{(j)}
    \right )\\
\end{align*}
